# Supplementary material for: Align, Then Adapt: Few-Shot fMRI Visual Reconstruction For New Subjects
Source: arXiv:2505.01670 source file (2026-10-24)
Supplement: Supplementary file 1 [file data_empirical.tex]

\section{Additional Experimental Results}\label{sec:ap_a}
\subsection{Best Candidate Image Selection: Additional Evaluation}\label{sec:ap_aone}
We conducted several experiments to demonstrate that our image selection strategy outperforms the baseline method in a limited data setting. Below we present our experimental results.

\begin{table}[h]
    \centering
    \caption{Comparison of performance on our data selection strategy with varying number of dimensions (singular values) for \textbf{Subject 2}. Our method
has not been optimized for low-level metrics, which are shown in gray for reference. 150 images were used for all the experiments in this table. }
    \vskip 0.1in
    \setlength{\tabcolsep}{2pt}  % Adjust the spacing between columns
      % Adjust the row height
    \footnotesize  % Reduce the font size
    \resizebox{0.65\textwidth}{!}{  % Resize the table to fit within the text width
    \begin{tabular}{cccccccccc}
        \toprule
        & \multicolumn{4}{c}{\textbf{Low-Level}} & \multicolumn{4}{c}{\textbf{High-Level}} \\
        \cmidrule(lr){2-5} \cmidrule(lr){6-9} 
        \textbf{Dimensions} & PixCorr $\uparrow$ & SSIM $\uparrow$ & Alex(2) $\uparrow$ & Alex(5) $\uparrow$ & Incep $\uparrow$ & CLIP $\uparrow$ & Eff $\downarrow$ & SwAV $\downarrow$ \\
        \midrule
        10 & {\color{gray} 0.099} & {\color{gray} 0.254} & {\color{gray} 74.27\%} & {\color{gray} \textbf{83.55\%}} & 75.20\% & \textbf{81.03\%} & 0.835 & 0.520 \\
        20 & {\color{gray} 0.105} & {\color{gray} 0.220} & {\color{gray} 73.06\%} & {\color{gray} 83.33\%} & \textbf{77.23\%} & 79.98\% & \textbf{0.828} & \textbf{0.508} \\
        30 & {\color{gray} \textbf{0.119}} & {\color{gray} \textbf{0.288}} & {\color{gray} \textbf{74.51\%}} & {\color{gray} 82.11\%} & 75.41\% & 79.12\% & 0.836 & 0.516 \\
        40 & {\color{gray} 0.103} & {\color{gray} 0.212} & {\color{gray} 72.22\%} & {\color{gray} 83.35\%} & 77.04\% & 79.44\% & 0.839 & 0.519 \\
        50 & {\color{gray} 0.107} & {\color{gray} 0.217} & {\color{gray} 73.73\%} & {\color{gray} 82.76\%} & 76.63\% & 78.75\% & 0.845 & 0.524 \\
        60 & {\color{gray} 0.101} & {\color{gray} 0.202} & {\color{gray} 72.91\%} & {\color{gray} 83.49\%} & 75.97\% & 79.97\% & 0.829 & 0.519 \\
        \bottomrule
    \end{tabular}
    }
    
    \label{tab:evs}
\end{table}
\begin{table}[h]
    \centering
    \caption{Comparison of performance on our data selection strategy with varying number of dimensions (singular values) for \textbf{Subject 5}. Our method has not been optimized for low-level metrics, which are shown in gray for reference. 150 images were used for all the
experiments in this table.}
    \vskip 0.1in
    \setlength{\tabcolsep}{2pt}  
      
    \footnotesize  
    \resizebox{0.65\textwidth}{!}{  
    \begin{tabular}{cccccccccc}
        \toprule
        & \multicolumn{4}{c}{\textbf{Low-Level}} & \multicolumn{4}{c}{\textbf{High-Level}} \\
        \cmidrule(lr){2-5} \cmidrule(lr){6-9} 
        \textbf{Dimensions} & PixCorr $\uparrow$ & SSIM $\uparrow$ & Alex(2) $\uparrow$ & Alex(5) $\uparrow$ & Incep $\uparrow$ & CLIP $\uparrow$ & Eff $\downarrow$ & SwAV $\downarrow$ \\
        \midrule
        10 & {\color{gray} \textbf{0.138}} & {\color{gray} \textbf{0.292}} & {\color{gray} 75.20\%} & {\color{gray} 83.81\%} & 78.62\% & 83.23\% & 0.818 & 0.525 \\
        20 & {\color{gray} 0.101} & {\color{gray} 0.241} & {\color{gray} 74.62\%} & {\color{gray} 84.26\%} & \textbf{80.11} & \textbf{83.97\%} & \textbf{0.797} & \textbf{0.487} \\
        30 & {\color{gray} 0.120} & {\color{gray} 0.276} & {\color{gray} \textbf{76.56\%}} & {\color{gray} 84.59\%} & 78.81\% & 83.03\% & 0.816 & 0.507 \\
        40 & {\color{gray} 0.119} & {\color{gray} 0.253} & {\color{gray} 76.01\%} & {\color{gray} \textbf{85.40\%}} & 79.16 & 83.56\% & 0.810 & 0.501 \\
        50 & {\color{gray} 0.106} & {\color{gray} 0.254} & {\color{gray} 74.85\%} & {\color{gray} 83.54\%} & 77.48\% & 81.83\% & 0.825 & 0.506 \\
        60 & {\color{gray} 0.116} & {\color{gray} 0.248} & {\color{gray} 75.32\%} & {\color{gray} 84.55\%} & 78.44\% & 82.22\% & 0.806 & 0.494 \\
        \bottomrule
    \end{tabular}
    }
    
    \label{tab:subj5}
\end{table}

\begin{table}[h]
    \centering
    \caption{ Comparison of performance on our data selection strategy with varying number of dimensions (singular values) for \textbf{Subject 7}. Our method has not been optimized for low-level metrics, which are shown in gray for reference. 150 images were used for all the
experiments in this table.}
    \vskip 0.1in
    \setlength{\tabcolsep}{2pt}  % Adjust the spacing between columns
      % Adjust the row height
    \footnotesize  % Reduce the font size
    \resizebox{0.65\textwidth}{!}{  % Resize the table to fit within the text width
    \begin{tabular}{cccccccccc}
        \toprule
        & \multicolumn{4}{c}{\textbf{Low-Level}} & \multicolumn{4}{c}{\textbf{High-Level}} \\
        \cmidrule(lr){2-5} \cmidrule(lr){6-9} 
        \textbf{Dimensions} & PixCorr $\uparrow$ & SSIM $\uparrow$ & Alex(2) $\uparrow$ & Alex(5) $\uparrow$ & Incep $\uparrow$ & CLIP $\uparrow$ & Eff $\downarrow$ & SwAV $\downarrow$ \\
        \midrule
        10 (150) & {\color{gray} 0.112} & {\color{gray} \textbf{0.272}} & {\color{gray} 72.60\%} & {\color{gray} 80.93\%} & 74.72\% & \textbf{79.09\%} & 0.840 & \textbf{0.509} \\
        20 (150) & {\color{gray} 0.095} & {\color{gray} 0.241} & {\color{gray} 69.75\%} & {\color{gray} 79.95\%} & 72.92\% & 77.51\% & 0.851 & 0.521 \\
        30 (150) & {\color{gray} 0.102} & {\color{gray} 0.258} & {\color{gray} 72.06v} & {\color{gray} 80.74\%} & 74.23\% & 77.92\% & 0.843 & 0.526 \\
        40 (150) & {\color{gray} \textbf{0.117}} & {\color{gray} 0.267} & {\color{gray} \textbf{73.23\%}} & {\color{gray} \textbf{80.99\%}} & 74.20\% & 78.15\% & 0.840 & 0.520 \\
        50 (150) & {\color{gray} 0.105} & {\color{gray} 0.220} & {\color{gray} 69.18\%} & {\color{gray} 78.17\%} & 70.75\% & 75.23\% & \textbf{0.860} & 0.533 \\
        60 (150) & {\color{gray} 0.103} & {\color{gray} 0.224} & {\color{gray} 69.43\%} & {\color{gray} 79.77\%} & \textbf{75.07\%} & 77.13\% & 0.839 & 0.528 \\
        \bottomrule
    \end{tabular}
    }
    
    \label{tab:subj7}
\end{table}

\begin{figure}[H]
    \centering
    \begin{subfigure}{0.4\columnwidth}
        \centering
        \includegraphics[width=\columnwidth]{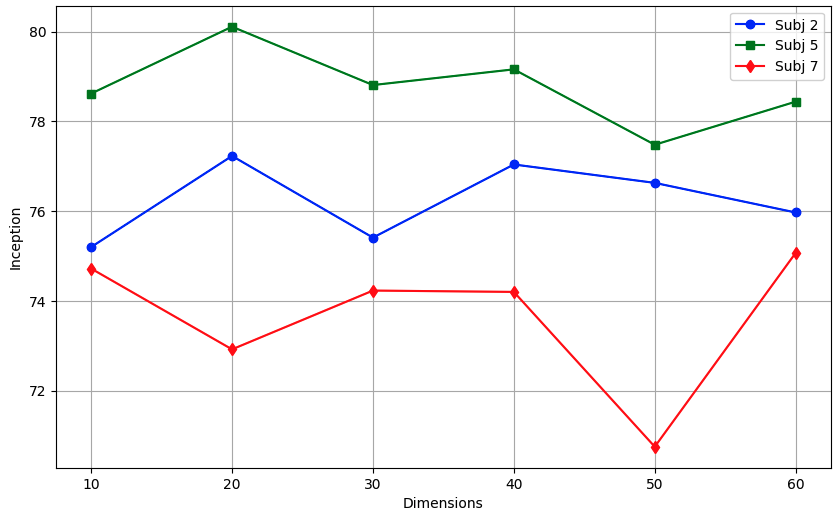}
    \end{subfigure}
    \begin{subfigure}{0.4\columnwidth}
        \centering
        \includegraphics[width=\columnwidth]{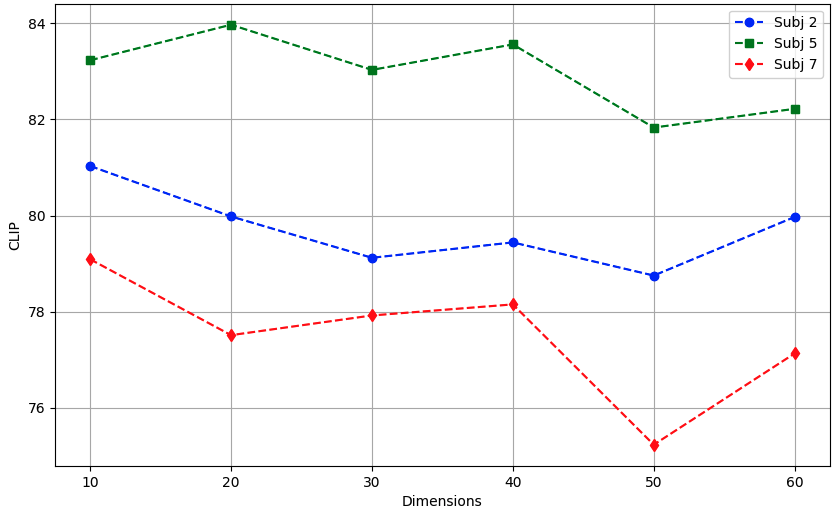}
    \end{subfigure}\hfill
    \caption{Comparison of the performance of the image selection strategy for different subjects. (a) Inception score with varying number of dimensions (b) CLIP score with varying number of dimensions.}
    \label{fig:ablat}
\end{figure}

\subsection{Impact of reference subject on performance} \label{sec:diff_reference}
We conducted additional experiments (Table \ref{tab:limitedcomparison_}) to explore the effect of different reference subjects on reconstruction results. We use subjects 2,5 and 7 as the reference and use subject 1 as the fine-tuning subject.
\begin{table}[h]
    \centering
    \caption{Quantitative results on fine tuning a new subject with limited data using different reference subjects. In this table we compare AAMax vs normal finetuning at 160 epochs only since AAMax significantly outperforms normal finetuning after 1 epoch of finetuning. }
    %\vspace{1.5pt}

    \vskip 0.1in
    \setlength{\tabcolsep}{2pt}  % Adjust the spacing between columns
      % Adjust the row height
    \footnotesize  % Reduce the font size
    \resizebox{\columnwidth}{!}{  % Resize the table to fit within the text width
    \begin{tabular}{lccccccccc}
        \toprule
        & \multicolumn{4}{c}{\textbf{Low-Level}} & \multicolumn{4}{c}{\textbf{High-Level}} \\
        \cmidrule(lr){2-5} \cmidrule(lr){6-9}
        \textbf{Method} & PixCorr $\uparrow$ & SSIM $\uparrow$ & Alex(2) $\uparrow$ & Alex(5) $\uparrow$ & Incep $\uparrow$ & CLIP $\uparrow$ & Eff $\downarrow$ & SwAV $\downarrow$\\
        \midrule
        Subj1 FT From Subj2 250 Normal E160    & {\color{gray}0.007} & {\color{gray}0.268} & {\color{gray}75.55\%} & {\color{gray}84.00\%} & 75.20\% & 74.60\% & 0.862 & 0.520 \\       
        Subj1 FT From Subj2 250 AAMAX E160     & \textbf{\color{gray}0.06} & \textbf{{\color{gray}0.277}} & \textbf{{\color{gray}81.13\%}} & \textbf{{\color{gray}88.99\%}} & \textbf{79.71\%} & \textbf{78.89\%} & \textbf{0.824} & \textbf{0.494} \\  
        \hline
        Subj1 FT From Subj5 250 Normal E160     & {\color{gray}0.094} & {\color{gray}0.239}  & {\color{gray}71.54\%}  & {\color{gray}80.10\%}         & 73.11\%        & 74.02\% & 0.875 & 0.537 \\ 
        Subj1 FT From Subj5 250 AAMAX E160      & \textbf{{\color{gray}0.105}}& \textbf{{\color{gray}0.259}} & \textbf{\color{gray}76.77\%}  & \textbf{{\color{gray}86.20\%}} & \textbf{80.08\%} & \textbf{80.14\%} & \textbf{0.828} & \textbf{0.496} \\  
        \hline
        Subj1 FT From Subj7 250 Normal E160     & {\color{gray}0.010} & {\color{gray}0.266} & {\color{gray}74.96\%} & {\color{gray}81.55\%} & 71.71\% & 73.72\% & 0.874 & 0.528 \\  
        Subj1 FT From Subj7 250 AAMAX E160      & \textbf{{\color{gray}0.012}} & \textbf{{\color{gray}0.283}} & \textbf{{\color{gray}79.58\%}} & \textbf{{\color{gray}87.78\%}} & \textbf{77.48\%} & \textbf{77.87\%} & \textbf{0.835} & \textbf{0.502} \\
        \bottomrule
    \end{tabular}
    }
    \label{tab:limitedcomparison_}
\end{table}
