# Supplementary material for: Align, Then Adapt: Few-Shot fMRI Visual Reconstruction For New Subjects
Source: arXiv:2505.01670 source file (2026-10-24)
Supplement: Supplementary file 2 [file limitations.tex]

\section{Limitations}\label{sec:limitations}
One key limitation of our approach is its reliance on a set of semantically similar or common stimuli. In addition, as with most of state of the art approaches \cite{scotti2024mindeye2}, we roughly need one hour of fMRI data per new subject. Another potential limitation of the proposed method is that the ultimate image fidelity hinges on the strengths and biases of the pre-trained diffusion model, meaning any generative shortcomings propagate into our outputs. Finally, variability and noise in the fMRI signals (e.g., scanner differences, low SNR) can further degrade adapter alignment and reconstruction accuracy.
